# Supplementary material for: Reconstructing Ultrametric Trees from Noisy Experiments
Source: arXiv:2206.07672 source file (2022-06-15)
Supplement: Supplementary file 1 [file appendix_old.tex]

\section{Proofs from Section~\ref{section:perfect_trees}}

\subsection{Proof of Claim~\ref{claim:local_sibling_ft}}
\label{subsection:pf_sibling_ft}


Now, consider some leaf $x \in S$, to show that $\expect{h_x} - \expect{w_x} = \Omega\left(\frac{w_{min}}{h(T)}\right)$, split the analysis into two cases - either $x \in L(T(q))$ or $x \notin L(T(q))$, i.e., whether or not $x$ is present in the sub-tree rooted at $q$, in other terms, whether or not $d(a,x) \le d(a,c)$. Consider the first case, where $d(a,x) \le d(a,c)$, represented in Fig~\ref{fig:ft_case1} and Fig~\ref{fig:ft_case1_alt}:

\begin{figure}[h]
    \centering
    \includegraphics[width = 8cm]{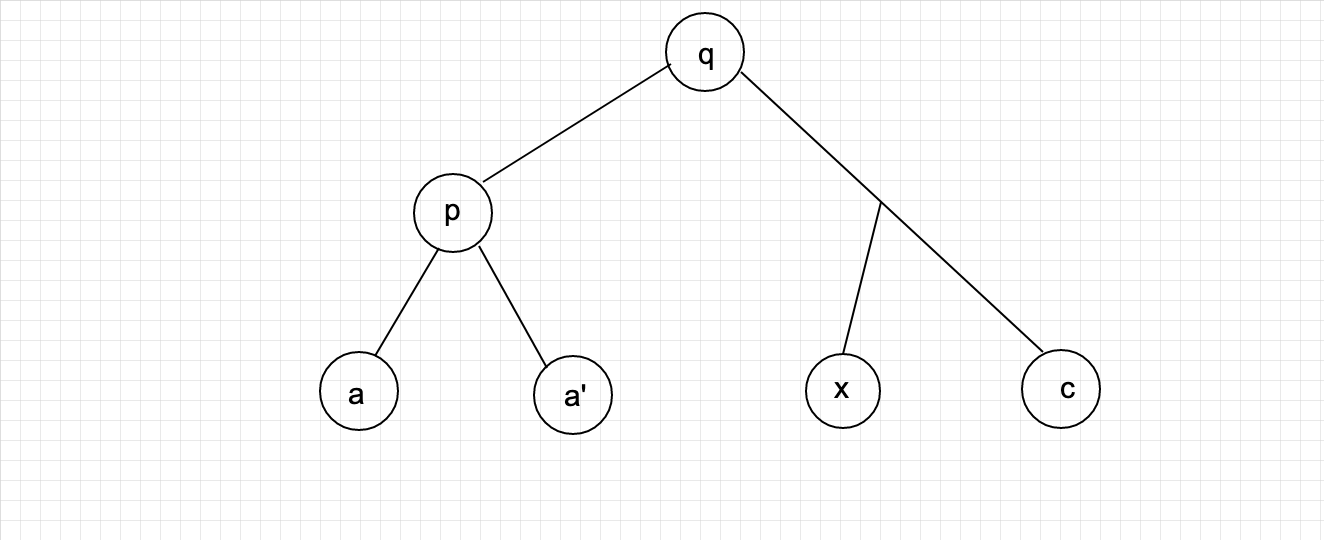}
    \caption{Case 1 (a) : $d(a,x) \le d(a,c)$}
    \label{fig:ft_case1}
\end{figure}

\begin{figure}[h]
    \centering
    \includegraphics[width=8cm]{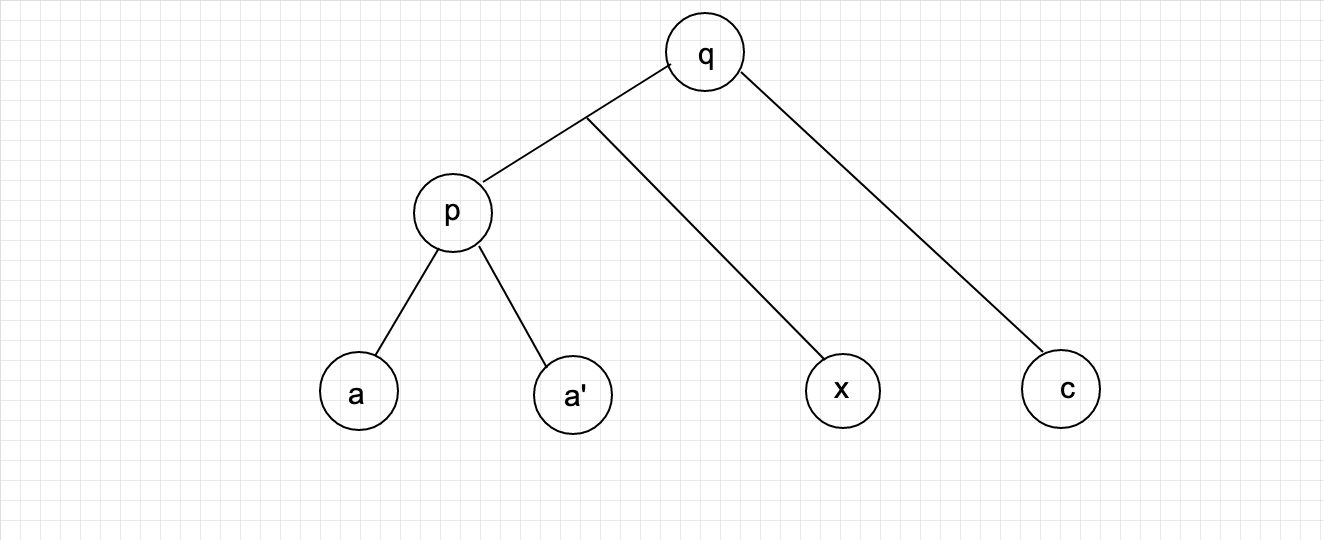}
    \caption{Case 1 (b) : $d(a,x) \le d(a,c)$}
    \label{fig:ft_case1_alt}
\end{figure}

The first sub-case is when $d(a,x) = d(a,c)$, i.e., when the least common ancestor of $c$ and $x$ is not $q$ (and is therefore in the same sub-tree of $q$ as $c$) , refer to Fig~\ref{fig:ft_case1}.

Let $d(a,a') = \alpha$, $d(a,x) = d(a',x) = d(a,c)  = \gamma$, $d(c,x) = \beta$. Note that $\alpha, \beta < \gamma$.

We have:

\begin{align*}
    \expect{h_x} &= \Pr[Q(a,a',x) = (a,a')]
    \\&= \frac{d(a,x) + d(a',x)}{2(d(a,a') + d(a,x) + d(a',x))}
   \\ &= \frac{2\gamma}{2(\alpha+2\gamma)}
\end{align*}

\begin{align*}
    \expect{w_x} &= \Pr[Q(a,c,x) = (a,c)]
    \\&= \frac{d(a,x) + d(c,x)}{2(d(a,c) + d(a,x) + d(c,x))}
   \\ &= \frac{\beta + \gamma}{2(\beta+2\gamma)}
\end{align*}

Taking the difference:

\begin{align*}
    \expect{h_x} - \expect{w_x} &= \frac{2\gamma (\beta+ 2 \gamma) - (\beta+\gamma)(\alpha+2\gamma)}{2(\alpha+2\gamma)(\beta+2\gamma)}
    \\&= \frac{2\gamma^2 - \alpha \beta - \alpha \gamma}{2(\alpha+2\gamma)(\beta+2\gamma)}
    \\&=\frac{(\gamma^2 - \alpha \beta) + (\gamma^2 - \alpha \gamma)}{2(\alpha+2\gamma)(\beta+2\gamma)}
    \\&\ge\frac{ (\gamma^2 - \alpha \gamma)}{2(\alpha+2\gamma)(\beta+2\gamma)}
    \\&\ge\frac{ \gamma(\gamma- \alpha )}{2(3\gamma)(3\gamma)}
    \\&\ge \frac{2w_{min}}{18h(T)}
\end{align*}


The other sub-case corresponds to $d(a,x) < d(a,c)$, i.e., the least common ancestor of $a$ and $x$ is below the internal vertex $q$, refer to Fig~\ref{fig:ft_case1_alt}.

Let $d(a,a') = \alpha$, $d(a,x) = d(a'x) = \beta$ and $d(a,c) = d(c,x) = \gamma$. Note that $\alpha < \beta < \gamma$.

We have:

\begin{align*}
    \expect{h_x} &= \Pr[Q(a,a',x) = (a,a')]
    \\&= \frac{d(a,x) + d(a',x)}{2(d(a,a') + d(a,x) + d(a',x))}
   \\ &= \frac{2\beta}{2(\alpha+2\beta)}
\end{align*}

\begin{align*}
    \expect{w_x} &= \Pr[Q(a,c,x) = (a,c)]
    \\&= \frac{d(a,x) + d(c,x)}{2(d(a,c) + d(a,x) + d(c,x))}
   \\ &= \frac{\beta + \gamma}{2(\beta+2\gamma)}
\end{align*}


Taking the difference:

\begin{align*}
    \expect{h_x} - \expect{w_x} &= \frac{2\beta (\beta+ 2 \gamma) - (\beta+\gamma)(\alpha+2\beta)}{2(\alpha+2\beta)(\beta+2\gamma)}
    \\&= \frac{2\beta \gamma -\beta \alpha - \gamma\alpha}{2(\alpha+2\beta)(\beta+2\gamma)}
    \\&=\frac{(\beta\gamma - \gamma \alpha) + (\beta \gamma - \beta \alpha)}{2(\alpha+2\beta)(\beta+2\gamma)}
    \\&\ge\frac{ (\beta \gamma - \gamma \alpha )}{2(\alpha+2\beta)(\beta+2\gamma)}
    \\&\ge\frac{ \gamma(\beta- \alpha )}{2(3\gamma)(3\gamma)}
    \\&\ge \frac{2w_{min}}{18h(T)}
\end{align*}

The second case is when $d(a,x) > d(a,c)$, depicted by Fig~\ref{fig:ft_case2}.
\begin{figure}[h]
    \centering
    \includegraphics[width=8cm]{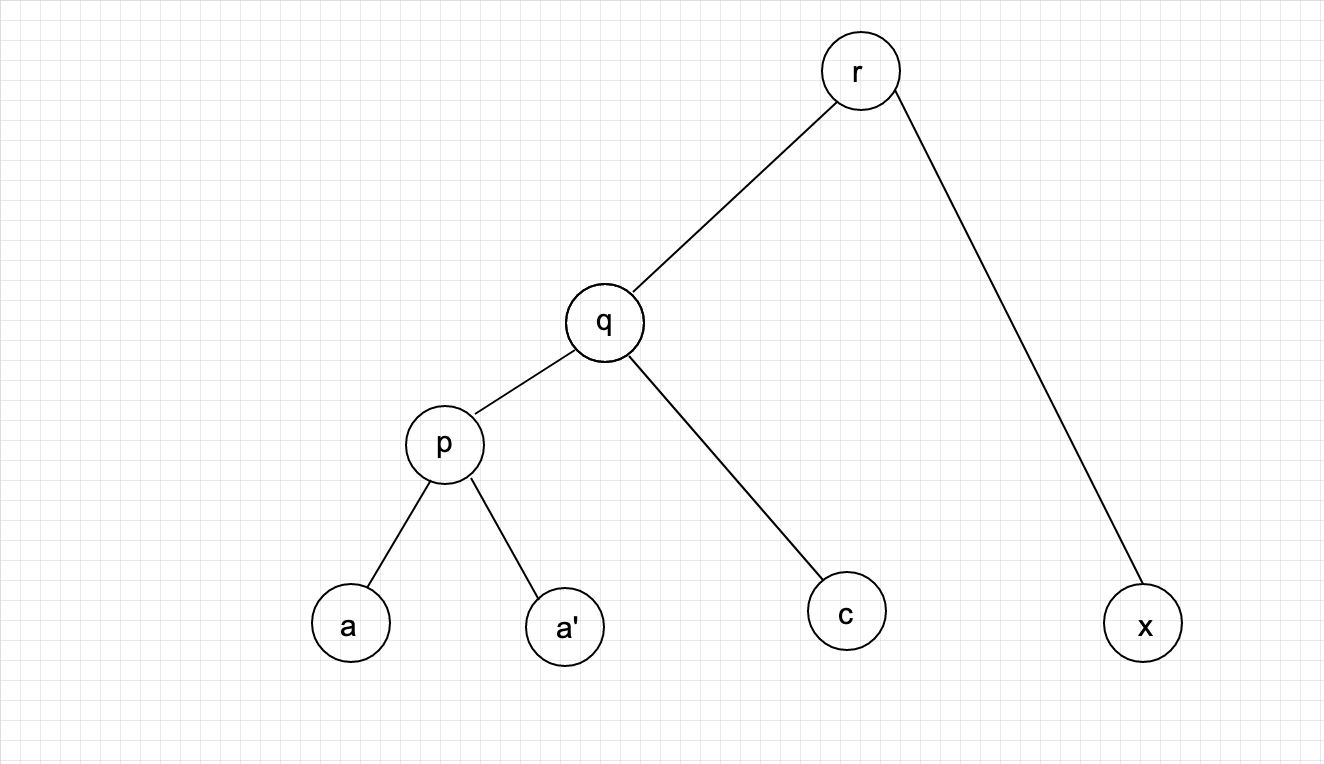}
    \caption{Case 2: $d(a,x) > d(a,c)$}
    \label{fig:ft_case2}
\end{figure}

Let $d(a,a') = \alpha$,$d(a,c) = \beta$ and $d(a,x) = d(a',x) = d(c,x) = \gamma$. Note that $\alpha < \beta < \gamma$.

We have:

\begin{align*}
    \expect{h_x} &= \Pr[Q(a,a',x) = (a,a')]
    \\&= \frac{d(a,x) + d(a',x)}{2(d(a,a') + d(a,x) + d(a',x))}
   \\ &= \frac{2\gamma}{2(\alpha+2\gamma)}
\end{align*}

\begin{align*}
    \expect{w_x} &= \Pr[Q(a,c,x) = (a,c)]
    \\&= \frac{d(a,x) + d(c,x)}{2(d(a,c) + d(a,x) + d(c,x))}
   \\ &= \frac{2\gamma}{2(\beta+2\gamma)}
\end{align*}


Taking the difference:

\begin{align*}
    \expect{h_x} - \expect{w_x} &= \frac{2\gamma (\beta+ 2 \gamma) - 2\gamma(\alpha+2\gamma)}{2(\alpha+2\gamma)(\beta+2\gamma)}
   \\ &= \frac{2\gamma (\beta -\alpha)}{2(\alpha+2\gamma)(\beta+2\gamma)}
   \\ &\ge \frac{2\gamma(\beta -\alpha)}{2(3\gamma)(3\gamma)}
   \\ &\ge \frac{4w_{min}}{9h(T)}
\end{align*}

This completes the proof of Claim~\ref{claim:local_sibling_ft}.

\subsection{Proof of Claim~\ref{claim:local_cousin_ft_reg1}}
\label{subsection:local_cousin_ft_reg1}

Consider any leaf $x \in F_{i-1}(a) \cup \{a\}$. Let $d(x,a') = \alpha$ and $d(x,c) = d(a'c) = \beta$ with $\alpha < \beta$.
\begin{figure}[h]
    \centering
    \includegraphics[width=8cm]{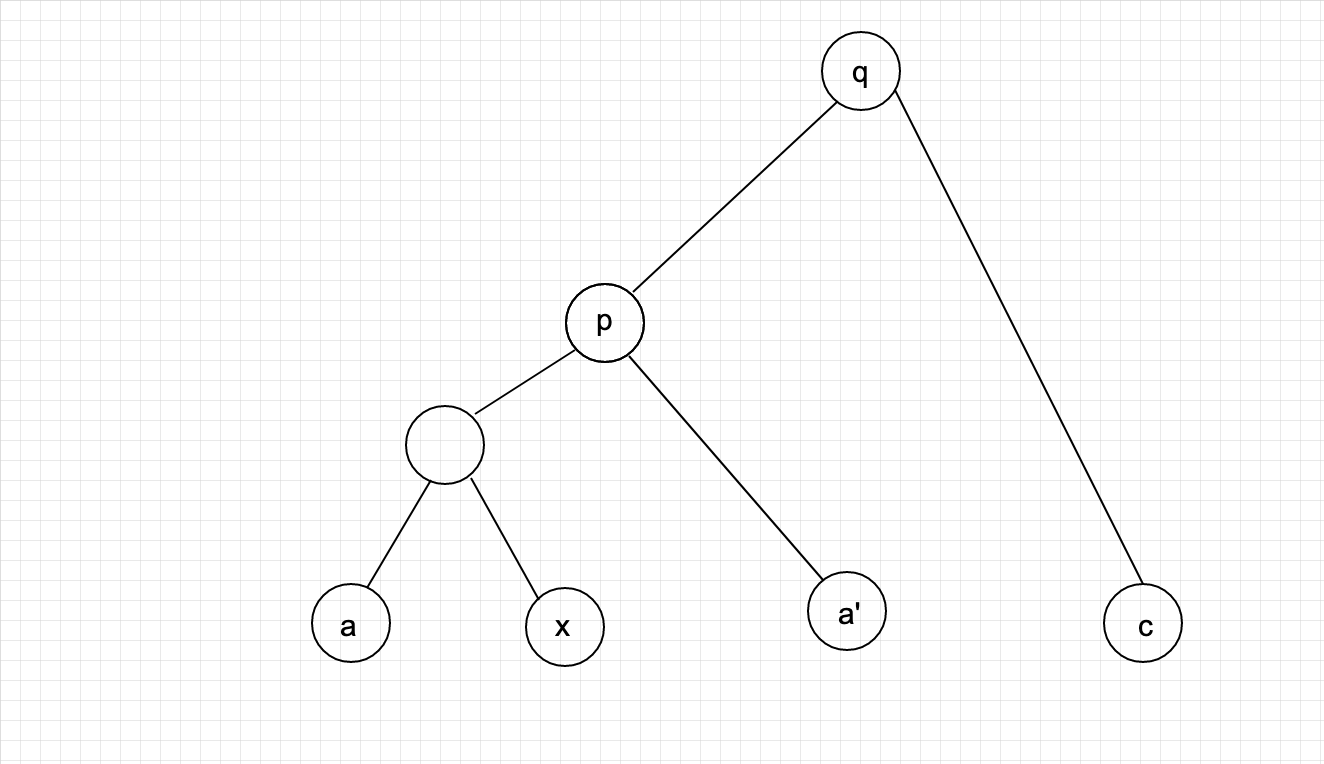}
    \caption{$x \in F_{i-1}(a) \cup \{a\}$}
    \label{fig:cousin_r2_ft}
\end{figure}

 Recall that $f_x$ is $1$ if $Q(x,a',c) = (x,a')$ and $g_x$ is $1$ if $Q(x,a',c) = (x,c)$. Thus, we have 
 \begin{align*}
     \expect{f_x} -\expect{g_x} &= \frac{2\beta}{2(\alpha +2\beta)} - \frac{\alpha + \beta}{2(\alpha +2\beta)}
     \\ &= \frac{\beta-\alpha}{2(\alpha+2\beta)}
     \\ &\ge \frac{w_{min}}{3h(T)}
 \end{align*}
